# Supplementary material for: Is Phase Shift Keying Optimal for Channels with Phase-Quantized Output?
Source: arXiv:2101.09896 ancillary file (2021-05-05)
Supplement: Supplementary file 1 [file supplement_mat.pdf]

# SUPPLEMENTARY MATERIALS - PROOFS

NEIL IRWIN BERNARDO, JINGGE ZHU, JAMIE EVANS

## A. Proof of Lemma 1

**Lemma 1.** *The function $W_y^{(b)}(\alpha,\theta)$ (or $W_y^{(b)}(u)$) satisfies the following properties:*

$$\begin{aligned} &(i) & W_y^{(b)}\left(\alpha,\theta+\frac{2\pi k}{2^b}\right) =& W_{y-k}^{(b)}\left(\alpha,\theta\right) & ,\forall k\in\mathbb{Z}\\ &(ii) & W_{2^{b-1}-y}^{(b)}\left(\alpha,\frac{\pi}{2^b}\right) =& W_{2^{b-1}+y}^{(b)}\left(\alpha,\frac{\pi}{2^b}\right) & \\ &(iii) & W_{2^{b-1}-y}^{(b)}\left(\alpha,0\right) =& W_{2^{b-1}-1+y}^{(b)}\left(\alpha,0\right) & \end{aligned}$$

*Proof.* Recall that the expression for $W_y^{(b)}(\alpha,\theta)$ is

$$W_y^{(b)}(\alpha,\theta) = \int_{\frac{2\pi}{2^b}y-\pi-\theta}^{\frac{2\pi}{2^b}(y+1)-\pi-\theta} p_{\Phi|A}(\phi|\alpha)\ d\phi, \tag{1}$$

where

$$\begin{aligned} p_{\Phi|A}(\phi|\alpha) =& \int_R p_{Z|U}\left(z=re^{j\phi}\middle|u=\sqrt{\alpha}\right)\ dr \\ =& \frac{e^{-\alpha}}{2\pi}+\frac{\sqrt{\alpha}\cos\phi e^{-\alpha\sin^2\phi}\left[1-Q\left(\sqrt{2\alpha}\cos\phi\right)\right]}{\sqrt{\pi}}. \end{aligned} \tag{2}$$

We can express $W_y^{(b)}(\alpha,\theta)$ as

$$\begin{aligned} W_y^{(b)}\left(\alpha,\theta+\frac{2\pi k}{2^b}\right) =& \int_{\frac{2\pi}{2^b}y-\pi-\theta-\frac{2\pi k}{2^b}}^{\frac{2\pi}{2^b}(y+1)-\pi-\theta-\frac{2\pi k}{2^b}} p_{\Phi|A}(\phi|\alpha)\ d\phi \\ =& \int_{\frac{2\pi}{2^b}(y-k)-\pi-\theta}^{\frac{2\pi}{2^b}(y+1-k)-\pi-\theta} p_{\Phi|A}(\phi|\alpha)\ d\phi \\ =& W_{y-k}^{(b)}\left(\alpha,\theta\right) \end{aligned}$$

which proves Lemma 1.i. For Lemma 1.ii, we have

$$\begin{aligned} W_{2^{b-1}-y}^{(b)}\left(\alpha,\frac{\pi}{2^b}\right) =& \int_{-\frac{2\pi y}{2^b}-\frac{\pi}{2^b}}^{-\frac{2\pi y}{2^b}+\frac{\pi}{2^b}} p_{\Phi|A}\left(\phi|\alpha\right)\ d\phi \\ =& \int_{\frac{2\pi y}{2^b}-\frac{\pi}{2^b}}^{\frac{2\pi y}{2^b}+\frac{\pi}{2^b}} p_{\Phi|A}\left(\phi'|\alpha\right)\ d\phi' \qquad (\text{Let } \phi'=-\phi) \end{aligned}$$

$$=W^{(b)}_{2^{b-1}+y}\left(\alpha, \frac{\pi}{2^b}\right),$$

where we obtain the last line by noting that the change of variable did not affect $p_{\Phi|A}(\phi|\alpha)$ since it is even-symmetric about $\phi = 0$. Finally, following the same arguments in the proof of Lemma 1.ii, lemma 1.iii is proven as follows:

$$\begin{aligned}
W^{(b)}_{2^{b-1}-y}(\alpha, 0) &= \int_{-\frac{2\pi y}{2^b}}^{-\frac{2\pi y}{2^b}+\frac{2\pi}{2^b}} p_{\Phi|A}(\phi|\alpha)\ d\phi \\
&= \int_{\frac{2\pi y}{2^b}-\frac{2\pi}{2^b}}^{\frac{2\pi y}{2^b}} p_{\Phi|A}(\phi'|\alpha)\ d\phi' \qquad (\text{Let } \phi' = -\phi) \\
&= W^{(b)}_{2^{b-1}-1+y}(\alpha, 0).
\end{aligned}$$

□

## B. Proof of Proposition 1

**Proposition 1.** *For any input distribution $F_U$, we define another input distribution as*

$$F^s_U = \frac{1}{2^b}\sum_{i=0}^{2^b-1} F_U(ue^{j\frac{2\pi i}{2^b}}),$$

*which is a $\frac{2\pi}{2^b}$-symmetric distribution. Then, $I(F^s_U) \geq I(F_U)$. Under this input distribution, $H(Y)$ is maximized and is equal to $b$.*

*Proof.* We first define the notations

$$H_{F_U}(Y) = -\int_{\mathbb{C}}\sum_{y=0}^{2^b-1} W^{(b)}_y(\alpha, \theta)\log p(y; F_U)\ dF_U$$

$$H_{F_U}(Y|U) = -\int_{\mathbb{C}}\sum_{y=0}^{2^b-1} W^{(b)}_y(\alpha, \theta)\log W^{(b)}_y(\alpha, \theta)\ dF_U,$$

where we used the subscript $F_U$ to note that the entropy and conditional entropy are induced by the input distribution in the subscript. We want to show that

$$H_{F^s_U}(Y) - H_{F^s_U}(Y|U) \geq H_{F_U}(Y) - H_{F_U}(Y|U) \quad \text{for any input distribution } F_U.$$

The conditional output entropy using $F^s_U$ is

$$\begin{aligned}
H_{F^s_U}(Y|U) &= -\int_{\mathbb{C}}\sum_{y=0}^{2^b-1} W^{(b)}_y(\alpha, \theta)\log W^{(b)}_y(\alpha, \theta)\ d\left[\frac{1}{2^b}\sum_{i=0}^{2^b-1} F_U(ue^{j\frac{2\pi i}{2^b}})\right] \\
&= -\frac{1}{2^b}\int_{\mathbb{C}}\sum_{y=0}^{2^b-1} W^{(b)}_y\left(\alpha, \theta - \frac{2\pi i}{2^b}\right)\log W^{(b)}_y\left(\alpha, \theta - \frac{2\pi i}{2^b}\right)\ dF_U(u)
\end{aligned}$$

Using Lemma 1.i and the circular structure of phase quantizer, it is easy to show that

$$\sum_{y=0}^{2^b-1} W_y^{(b)}\left(\alpha, \theta - \frac{2\pi i}{2^b}\right) \log W_y^{(b)}\left(\alpha, \theta - \frac{2\pi i}{2^b}\right) = \sum_{y=0}^{2^b-1} W_y^{(b)}(\alpha, \theta) \log W_y^{(b)}(\alpha, \theta).$$

Consequently, $H_{F_U^s}(Y|U)$ can be simplified to

$$H_{F_U^s}(Y|U) = -\frac{1}{2^b}\sum_{i=0}^{2^b-1}\int_{\mathbb{C}}\sum_{y=0}^{2^b-1} W_y^{(b)}(\alpha, \theta) \log W_y^{(b)}(\alpha, \theta)\ dF_U = H_{F_U}(Y|U).$$

For the output PMF, we examine the PMF $p(y; F_U^s)$:

$$\begin{aligned} p(y; F_U^s) &= \int_{\mathbb{C}} W_y^{(b)}(\alpha, \theta)\ d\left[\frac{1}{2^b}\sum_{i=0}^{2^b-1} F_U(ue^{j\frac{2\pi i}{2^b}})\right] \\ &= \frac{1}{2^b}\int_{\mathbb{C}} \underbrace{\sum_{i=0}^{2^b-1} W_y^{(b)}(\alpha, \theta)}_{=1}\ dF_U(ue^{j\frac{2\pi i}{2^b}}) \\ &= \frac{1}{2^b}\int_{\mathbb{C}} dF_U(ue^{j\frac{2\pi i}{2^b}}) = \frac{1}{2^b} \end{aligned}$$

Thus, the PMF of $Y$ is a uniform distribution and also maximizes the output entropy. More specifically, the output entropy is $H_{F_U^s}(Y) = b$. This also implies that $I(F_U^s) \geq I(F_U)$. □

## C. Proof of Lemma 2

**Lemma 2.** *The function $H(Y|U = \sqrt{\alpha}e^{j\theta})$ is decreasing on $\alpha$ for all $\theta \in \left[0, \frac{2\pi}{2^b}\right)$ and $b \geq 1$.*

*Proof.* Note that the special case of $b = 1$ is already proven in [1, Appendix D] and the proof can be readily extended to $b = 2$ by treating this case as two 1-bit quantizers for I and Q. Thus, we only need to consider $b \geq 3$. Suppose we define the function

$$w(\alpha, \theta, b) = H(Y|U = \sqrt{\alpha}e^{j\theta})$$

To show that $w(\alpha, \theta, b)$ is decreasing, we consider the first-order derivative of $w(\alpha, \theta, b)$ with respect to $\alpha$, which can be written as

$$\begin{aligned} \frac{\partial w(\alpha, \theta, b)}{\partial \alpha} &= -\sum_{y=0}^{2^b-1} \frac{1 + \ln W_y^{(b)}(\alpha, \theta)}{\ln 2} \cdot \frac{\partial W_y^{(b)}(\alpha, \theta)}{\partial \alpha} \\ &= -\sum_{y \neq 2^{b-1}} \frac{1 + \ln W_y^{(b)}(\alpha, \theta)}{\ln 2} \frac{\partial W_y^{(b)}(\alpha, \theta)}{\partial \alpha} - \frac{1 + \ln W_{2^{b-1}}^{(b)}(\alpha, \theta)}{\ln 2} \frac{\partial W_{2^{b-1}}^{(b)}(\alpha, \theta)}{\partial \alpha} \\ &= \sum_{y \neq 2^{b-1}} \frac{\partial W_y^{(b)}(\alpha, \theta)}{\partial \alpha} \underbrace{\left[\log \frac{W_{2^{b-1}}^{(b)}(\alpha, \theta)}{W_y^{(b)}(\alpha, \theta)}\right]}_{\geq 0}. \end{aligned} \tag{3}$$

The first line follows from the chain rule of differentiation. The third line follows from some algebraic manipulation and the fact that $\sum_{\text{all } y} W_y^{(b)}(\alpha,\theta) = 1$ so

$$W_{2^{b-1}}^{(b)}(\alpha,\theta) = 1 - \sum_{y\neq 2^{b-1}} W_y^{(b)}(\alpha,\theta) \Longrightarrow \frac{\partial W_{2^{b-1}}^{(b)}(\alpha,\theta)}{\partial\alpha} = -\sum_{y\neq 2^{b-1}} \frac{\partial W_y^{(b)}(\alpha,\theta)}{\partial\alpha}. \tag{4}$$

Moreover, $W_{2^{b-1}}(\alpha,\theta) \geq W_y(\alpha,\theta)\ \forall y \neq 2^{b-1}$ since $\theta \in \mathcal{R}_{2^{b-1}}^{(\mathrm{PH})}$. Because of Lemma 8 (See Section J) and the fact that $p_{\Phi|A}(\phi|\alpha)$ is non-decreasing (non-increasing) function of $\phi$ for $\phi < 0$ ($\phi > 0$), there exists two integers $y_0^{(1)} \leq 2^{b-1}$ and $y_1^{(1)} \geq 2^{b-1}$ such that we can define the integer sets $\mathcal{Y}_1 = [y_0^{(1)}, y_1^{(1)}]$ and $\mathcal{Y}_1^c = [0, y_0^{(1)}-1] \cup [y_1^{(1)}+1, 2^b-1]$ satisfying

$$\text{(i) } \frac{\partial W_y^{(b)}(\alpha,\theta)}{\partial\alpha} \geq 0, y \in \mathcal{Y}_1,$$
$$\text{(ii) } \frac{\partial W_y^{(b)}(\alpha,\theta)}{\partial\alpha} < 0, y \in \mathcal{Y}_1^c, \text{ and}$$
$$\text{(ii) } \min_{k\in\mathcal{Y}_1}\{W_k^{(b)}(\alpha,\theta)\} \geq \max_{j\in\mathcal{Y}_1^c}\{W_j^{(b)}(\alpha,\theta)\}.$$

Given these, $\frac{\partial w(\alpha,\theta,b)}{\partial\alpha}$ can be upper bounded as

$$\begin{aligned}
\frac{\partial w(\alpha,\theta,b)}{\partial\alpha} &= \sum_{y\in\mathcal{Y}_1\setminus\{2^{b-1}\}} \underbrace{\frac{\partial W_y^{(b)}(\alpha,\theta)}{\partial\alpha}}_{\geq 0}\left[\log\frac{W_{2^{b-1}}^{(b)}(\alpha,\theta)}{W_y^{(b)}(\alpha,\theta)}\right] + \sum_{y\in\mathcal{Y}_1^c} \underbrace{\frac{\partial W_y^{(b)}(\alpha,\theta)}{\partial\alpha}}_{\leq 0}\left[\log\frac{W_{2^{b-1}}^{(b)}(\alpha,\theta)}{W_y^{(b)}(\alpha,\theta)}\right] \\
&\leq K_1 \sum_{y\in\mathcal{Y}_1\setminus\{2^{b-1}\}} \frac{\partial W_y^{(b)}(\alpha,\theta)}{\partial\alpha} + K_2 \sum_{y\in\mathcal{Y}_1^c} \frac{\partial W_y^{(b)}(\alpha,\theta)}{\partial\alpha} \\
&\leq K_2 \sum_{y\neq 2^{b-1}} \frac{\partial W_y^{(b)}(\alpha,\theta)}{\partial\alpha} \\
&= -K_2 \frac{\partial W_{2^{b-1}}^{(b)}(\alpha,\theta)}{\partial\alpha},
\end{aligned}$$

where $K_1$ and $K_2$ are

$$K_1 = \log\frac{W_{2^{b-1}}^{(b)}(\alpha,\theta)}{\min_{y\in\mathcal{Y}_1\setminus\{2^{b-1}\}}\{W_y^{(b)}(\alpha,\theta)\}} \text{ and } K_2 = \log\frac{W_{2^{b-1}}^{(b)}(\alpha,\theta)}{\max_{y\in\mathcal{Y}_1^c}\{W_y^{(b)}(\alpha,\theta)\}}. \tag{5}$$

The first line is obtained by placing all the positive terms in the first summation and all the negative terms in the second summation. The upper bound in the second line is obtained from using $K_1$ and $K_2$ for the $\log(\cdot)$ terms of the first and second summations, respectively. The third line follows from the fact that $K_1 < K_2$ so replacing $K_1$ by $K_2$ increases the positive terms. The last line follows from (4). The proof is completed by showing that $W_{2^{b-1}}^{(b)}(\alpha,\theta)$ is an increasing function of $\alpha$ for $b \geq 3$ (see Section K). □

## D. Proof of Lemma 3

**Lemma 3.** *The function $H(Y|U = \sqrt{\alpha}e^{j\theta})$ is convex on $\alpha$ for all $\theta \in \left[0, \frac{2\pi}{2^b}\right)$ and $b \geq 1$.*

*Proof.* Note that the special case of $b = 1$ is already proven in [1, Appendix D] and the proof can be readily extended to $b = 2$ by treating this case as two 1-bit quantizers for I and Q (as in the method of [2]). Thus, we only need to consider $b \geq 3$. To show that $w(\alpha, \theta, b)$ is convex, we show that its second-order derivative with respect to $\alpha$ is non-positive. That is,

$$\frac{\partial^2 w(\alpha,\theta)}{\partial \alpha^2} = \sum_{y \neq 2^{b-1}} \frac{\partial^2 W_y^{(b)}(\alpha,\theta)}{\partial \alpha^2} \log_2 \left\{ \frac{W_{2^{b-1}}^{(b)}(\alpha,\theta)}{W_y^{(b)}(\alpha,\theta)} \right\} - \sum_{y=0}^{2^b-1} \frac{1}{W_y^{(b)}(\alpha,\theta)} \frac{\partial W_y^{(b)}(\alpha,\theta)}{\partial \alpha}, \tag{6}$$

which is obtained by applying chain rule of differentiation to (3), is greater than or equal to zero. This can be lower bounded as

$$\begin{aligned}
\frac{\partial^2 w(\alpha,\theta)}{\partial \alpha^2} =& -\sum_{y \in \mathcal{Y}_1} \frac{1}{W_y^{(b)}(\alpha,\theta)} \underbrace{\frac{\partial W_y^{(b)}(\alpha,\theta)}{\partial \alpha}}_{\geq 0} + \sum_{y \in \mathcal{Y}_1^c} \frac{1}{W_y^{(b)}(\alpha,\theta)} \underbrace{\left[ -\frac{\partial W_y^{(b)}(\alpha,\theta)}{\partial \alpha} \right]}_{\geq 0} \\
&+ \sum_{y \neq 2^{b-1}} \frac{\partial^2 W_y^{(b)}(\alpha,\theta)}{\partial \alpha^2} \log_2 \left\{ \frac{W_{2^{b-1}}^{(b)}(\alpha,\theta)}{W_y^{(b)}(\alpha,\theta)} \right\} \\
\geq& \sum_{y \in \mathcal{Y}_1} K_1' \underbrace{\left[ -\frac{\partial W_y^{(b)}(\alpha,\theta)}{\partial \alpha} \right]}_{\leq 0} + \sum_{y \in \mathcal{Y}_1^c} K_2' \underbrace{\left[ -\frac{\partial W_y^{(b)}(\alpha,\theta)}{\partial \alpha} \right]}_{\geq 0} \\
&+ \sum_{y \neq 2^{b-1}} \frac{\partial^2 W_y^{(b)}(\alpha,\theta)}{\partial \alpha^2} \log_2 \left\{ \frac{W_{2^{b-1}}^{(b)}(\alpha,\theta)}{W_y^{(b)}(\alpha,\theta)} \right\} \\
\geq& K_2' \underbrace{\sum_{y=0}^{2^{b-1}-1} \left[ -\frac{\partial W_y^{(b)}(\alpha,\theta)}{\partial \alpha} \right]}_{=0} + \sum_{y \neq 2^{b-1}} \frac{\partial^2 W_y^{(b)}(\alpha,\theta)}{\partial \alpha^2} \log_2 \left\{ \frac{W_{2^{b-1}}^{(b)}(\alpha,\theta)}{W_y^{(b)}(\alpha,\theta)} \right\},
\end{aligned}$$

where $\mathcal{Y}_1$ and $\mathcal{Y}_1^c$ are integer sets defined in Section C and $K_1'$,$K_2'$ are

$$K_1' = \frac{1}{\min_{y \in \mathcal{Y}_1} \{ W_y^{(b)}(\alpha,\theta) \}} \text{ and } K_2' = \frac{1}{\max_{y \in \mathcal{Y}_1^c} \{ W_y^{(b)}(\alpha,\theta) \}}. \tag{7}$$

The first line follows from placing all the positive $\frac{\partial^2 W_y^{(b)}(\alpha,\theta)}{\partial \alpha^2}$ terms in the first summation and all the negative $\frac{\partial^2 W_y^{(b)}(\alpha,\theta)}{\partial \alpha^2}$ terms in the second summation. The second inequality follows from using $K_1'$ and $K_2'$. The third inequality follows from the fact that $K_1' < K_2'$ so replacing $K_1'$ by $K_2'$ increases the negative terms. Consequently, the first summation term in the last line becomes zero because of (4).

Because of Lemma 9 (See Section L) and the fact that $p_{\Phi|A}(\phi|\alpha)$ is a non-decreasing (non-increasing) function of $\phi$ for $\phi < 0$ ($\phi > 0$), there exists two integers $y_0^{(2)} \leq 2^{b-1}$ and $y_1^{(2)} \geq 2^{b-1}$ such that we can define the integer sets $\mathcal{Y}_2 = [y_0^{(2)}, y_1^{(2)}]$ and $\mathcal{Y}_2^c = [0, y_0^{(2)} - 1] \cup [y_1^{(2)} + 1, 2^b - 1]$ satisfying

$$\text{(i) } \frac{\partial^2 W_y^{(b)}(\alpha,\theta)}{\partial \alpha^2} \leq 0, y \in \mathcal{Y}_2,$$

(ii) $\dfrac{\partial^2 W_y^{(b)}(\alpha,\theta)}{\partial\alpha^2} > 0, y \in \mathcal{Y}_2^c,$ and

(ii) $\min_{k\in\mathcal{Y}_2}\{W_k^{(b)}(\alpha,\theta)\} \geq \max_{j\in\mathcal{Y}_2^c}\{W_j^{(b)}(\alpha,\theta)\}$.

Using a similar approach in Section C, we define two constants, $K_1''$ and $K_2''$, which are

$$K_1'' = \log \frac{W_{2^{b-1}}^{(b)}(\alpha,\theta)}{\min_{y\in\mathcal{Y}_2\setminus\{2^{b-1}\}}\{W_y^{(b)}(\alpha,\theta)\}} \text{ and } K_2'' = \log \frac{W_{2^{b-1}}^{(b)}(\alpha,\theta)}{\max_{y\in\mathcal{Y}_2^c}\{W_y^{(b)}(\alpha,\theta)\}} \tag{8}$$

and get the following lower bound for $\frac{\partial^2 w(\alpha,\theta)}{\partial\alpha^2}$:

$$\begin{aligned}
\frac{\partial^2 w(\alpha,\theta)}{\partial\alpha^2} \geq & \sum_{y\neq 2^{b-1}} \frac{\partial^2 W_y^{(b)}(\alpha,\theta)}{\partial\alpha^2} \log_2\left\{\frac{W_{2^{b-1}}^{(b)}(\alpha,\theta)}{W_y^{(b)}(\alpha,\theta)}\right\} \\
\geq & K_2'' \sum_{y\neq 2^{b-1}} \frac{\partial^2 W_y^{(b)}(\alpha,\theta)}{\partial\alpha^2} \\
= & -K_2'' \cdot \frac{\partial^2 W_{2^{b-1}}^{(b)}(\alpha,\theta)}{\partial\alpha^2},
\end{aligned}$$

where the last line follows from extending (4) to second-order derivatives. Thus, the proof is completed by showing that $W_{2^{b-1}}^{(b)}(\alpha,\theta)$ is a concave function of $\alpha$ for $b \geq 3$ (see Section M). □

## E. Proof of Lemma 4

**Lemma 4.** *The set $\Omega_\Theta^s$ is convex and weakly compact.*

*Proof.* The distributions contained in $\Omega_\Theta^s$ have a compact support. As such, its compactness in the weak* topology is a consequence of Banach-Alaoglu Theorem [3]. To prove the convexity of the set, we draw two $\frac{2\pi}{2^b}$-symmetric distributions, $F_{\Theta,1}^s$ and $F_{\Theta,2}^s$, such that

$$\begin{aligned}
F_{\Theta,1}^s = & \frac{1}{2^b}\sum_{i=0}^{2^b-1} F_{\Theta,1}\left(\theta + \frac{2\pi i}{2^b} \mod 2\pi\right) \\
F_{\Theta,2}^s = & \frac{1}{2^b}\sum_{i=0}^{2^b-1} F_{\Theta,2}\left(\theta + \frac{2\pi i}{2^b} \mod 2\pi\right)
\end{aligned}$$

for some arbitrary $F_{\Theta,1}$ and $F_{\Theta,2}$ (not necessarily symmetric). For any $\lambda \in [0,1]$, we can define another input distribution $F_{\Theta,\lambda}^s = \lambda F_{\Theta,1}^s + (1-\lambda)F_{\Theta,2}^s$ as

$$\begin{aligned}
F_{\Theta,\lambda}^s = & \frac{1}{2^b}\sum_{i=0}^{2^b-1} \lambda F_{\Theta,1}\left(\theta + \frac{2\pi i}{2^b} \mod 2\pi\right) + (1-\lambda)F_{\Theta,2}\left(\theta + \frac{2\pi i}{2^b} \mod 2\pi\right) \\
= & \frac{1}{2^b}\sum_{i=0}^{2^b-1} F_{\Theta,\lambda}\left(\theta + \frac{2\pi i}{2^b} \mod 2\pi\right)
\end{aligned}$$

for some circular distribution $F_{\Theta,\lambda} = \lambda F_{\Theta,1} + (1-\lambda)F_{\Theta,2}$. Noting that $F_{\Theta,\lambda}^s \in \Omega_\Theta^s$ concludes the proof. □

## F. Proof of Lemma 5

**Lemma 5.** *The function*

$$\bar{w}(F_\Theta) = \mathbb{E}_\Theta\left[-\sum_{y=0}^{2^b-1} W_y^{(b)}(P',\theta)\log W_y^{(b)}(P',\theta)\right]$$

*is convex and weakly differentiable on $F_\Theta$.*

*Proof.* The convexity of $\bar{w}(F_\Theta)$ follows from the fact that it can be expressed as

$$\bar{w}(F_\Theta) = b - I(F_\Theta),$$

where $I(F_\Theta)$ is the mutual information induced by the distribution $F_\Theta$. Since mutual information is a concave functional of the input distribution [4, Theorem 2.7.4], $\bar{w}(F_\Theta)$ is convex.

The function is weakly differentiable if for any $F_\Theta^0 \in \Omega_\Theta^s$, the weak derivative

$$\bar{w}'_{F_\Theta^0}(F_\Theta) = \lim_{\lambda\to 0}\frac{\bar{w}\left((1-\lambda)F_\Theta^0 + \lambda F_\Theta\right) - \bar{w}(F_\Theta^0)}{\lambda} \tag{9}$$

exists for all $F_\Theta \in \Omega_\Theta^s$. Suppose we let $F_\Theta^\lambda = (1-\lambda)F_\Theta^0 + \lambda F_\Theta$. It can be shown that the weak derivative

$$\begin{aligned}
\bar{w}'_{F_\Theta^0}(F_\Theta) &= \lim_{\lambda\to 0}\frac{\bar{w}\left(F_\Theta^\lambda\right) - \bar{w}(F_\Theta^0)}{\lambda}\\
&= \lim_{\lambda\to 0}\frac{(1-\lambda)\bar{w}\left(F_\Theta^0\right) + \lambda\bar{w}\left(F_\Theta\right) - \bar{w}(F_\Theta^0)}{\lambda}\\
&= \lim_{\lambda\to 0}\frac{\lambda\left[\bar{w}\left(F_\Theta\right) - \bar{w}\left(F_\Theta^0\right)\right]}{\lambda}\\
&= \bar{w}\left(F_\Theta\right) - \bar{w}\left(F_\Theta^0\right)
\end{aligned}$$

exists because both terms are finite. □

## G. Proof of Lemma 6

**Lemma 6.** *The support set of $F_\Theta^*$ is discrete and contains at most $2^b$ points.*

*Proof.* The set $\Omega_\Theta^s$ can be expressed as

$$\Omega_\Theta^s = \{F_\Theta \in \Omega_\Theta | p(y;F_\Theta) = 1/2^b\},$$

where $\Omega_\Theta$ is the set of all probability distributions with support $[-\pi,\pi]$ and $p(y;F_\Theta)$ is the output PMF induced by the input distribution with amplitude $\sqrt{\alpha} = \sqrt{P}$ and phase distribution $F_\Theta$. With $F_\Theta \in \Omega_\Theta^s$, the capacity can be written as

$$C = b - \inf_{F_\Theta\in\Omega_\Theta^s}\left\{\int_{\text{supp}(F_\Theta)} w\left(\frac{|g_{\text{LoS}}|^2P}{\sigma^2},\theta,b\right)\,dF_\Theta\right\}.$$

The mutual information is a sum of a constant term and a linear functional term over the set $\Omega_\Theta^s$. As a result, it achieves a maximum at an extreme point of $\Omega_\Theta^s$ and this input distribution is $F_\Theta^*$. We can consider $\Omega_\Theta^s$ as intersection of $\Omega_\Theta$ and $2^b-1$ hyperplanes given by

$$\mathcal{H}_y : \int_{\mathcal{M}} W_y^{(b)}\left(\frac{|g_{\text{LoS}}|^2P}{\sigma^2},\theta,b\right)\,dF_U = \frac{1}{2^b} \qquad ,\forall y\in[0,2^b-2]$$

(defining $\mathcal{H}_{2^b-1}$ is redundant since the probability of all mass points should sum up to 1). By applying Dubin's Theorem [5] in a similar manner as in [6], the optimal distribution $F_\Theta^*$ is a convex combination of at most $2^b$ extreme points of $\Omega_\Theta^s$. These extreme points are the set of at most $L$ unit masses $\{\delta(\theta_i)\}_{i=1}^{i=L}$, where $\theta_i \in [-\pi, \pi]$ and $L \leq 2^b$. ☐

## H. Proof of Proposition 3

**Proposition 3.** *The set containing the angles of the optimum mass points $u^* \in F_U^*$ is given by*

$$\theta^* = \left\{ \frac{2\pi(k+0.5)}{2^b} \right\}_{k=0}^{2^b-1}.$$

*Proof.* In the main text, we defined the optimality condition

$$C - b - \sum_{y=0}^{2^b-1} W_y^{(b)}(P', \theta) \log W_y^{(b)}(P', \theta) \geq 0, \tag{10}$$

Suppose we let a function $\mathcal{L}(\theta)$ be

$$\mathcal{L}(\theta) = C - b - \sum_{y=0}^{2^b-1} W_y^{(b)}(P', \theta) \log W_y^{(b)}(P', \theta)$$

(i.e. the LHS of equation (10)). Then an optimal $\theta$ should satisfy the following stationary condition

$$\left. \frac{\partial \mathcal{L}(\theta)}{\partial \theta} \right|_{\theta=\theta^*} = 0,$$

The expression for $\frac{\partial \mathcal{L}(\theta)}{\partial \theta}$ can be explicitly written as

$$\frac{\partial \mathcal{L}(\theta)}{\partial \theta} = \sum_{y \neq 2^{b-1}} \frac{\partial W_y^{(b)}(P', \theta)}{\partial \theta} \log \left[ \frac{W_{2^{b-1}}^{(b)}(P', \theta)}{W_y^{(b)}(P', \theta)} \right], \tag{11}$$

obtained using chain rule of differentiation and the fact that

$$\sum_{y=0}^{2^{b-1}} \frac{\partial W_y^{(b)}(P', \theta)}{\partial \theta} = 0$$

since $\sum_{y=0}^{2^{b-1}} W_y^{(b)}(P', \theta) = 1$. We can rewrite (11) as

$$\begin{aligned} \frac{\partial \mathcal{L}(\theta)}{\partial \theta} = \sum_{y=1}^{y=2^{b-1}-1} & \left\{ \frac{\partial W_{2^{b-1}-y}^{(b)}(P', \theta)}{\partial \theta} \log \left[ \frac{W_{2^{b-1}}^{(b)}(P', \theta)}{W_{2^{b-1}-y}^{(b)}(P', \theta)} \right] \right. \\ & \left. + \frac{\partial W_{2^{b-1}+y}^{(b)}(P', \theta)}{\partial \theta} \log \left[ \frac{W_{2^{b-1}}^{(b)}(P', \theta)}{W_{2^{b-1}+y}^{(b)}(P', \theta)} \right] \right\} \\ & + \frac{\partial W_0^{(b)}(P', \theta)}{\partial \theta} \log \left[ \frac{W_{2^{b-1}}^{(b)}(P', \theta)}{W_0^{(b)}(P', \theta)} \right]. \end{aligned} \tag{12}$$

Suppose $\theta = \frac{\pi}{2^b}$. We can apply Leibniz integral rule to get

$$
\begin{aligned}
\frac{\partial W^{(b)}_{2^{b-1}-y}(P',\theta)}{\partial\theta}\Big|_{\theta=\frac{\pi}{2^b}} =& p_{\Phi|A}\left(-\frac{2\pi(y+0.5)}{2^b}\Big|P'\right) - p_{\Phi|A}\left(\frac{2\pi(y-0.5)}{2^b}\Big|P'\right)\\
\frac{\partial W^{(b)}_{2^{b-1}+y}(P',\theta)}{\partial\theta}\Big|_{\theta=\frac{\pi}{2^b}} =& p_{\Phi|A}\left(\frac{2\pi(y-0.5)}{2^b}\Big|P'\right) - p_{\Phi|A}\left(\frac{2\pi(y+0.5)}{2^b}\Big|P'\right)\\
\frac{\partial W^{(b)}_{0}(P',\theta)}{\partial\theta}\Big|_{\theta=\frac{\pi}{2^b}} =& p_{\Phi|A}\left(-\frac{\pi}{2^b}\Big|P'\right) - p_{\Phi|A}\left(\frac{\pi}{2^b}\Big|P'\right)
\end{aligned}
$$

Due to even-symmetry of $p_{\Phi|A}(\phi|\alpha)$, we have

$$
\begin{aligned}
\frac{\partial W^{(b)}_{2^{b-1}-y}(P',\theta)}{\partial\theta}\Big|_{\theta=\frac{\pi}{2^b}} =& -\frac{\partial W^{(b)}_{2^{b-1}+y}(P',\theta)}{\partial\theta}\Big|_{\theta=\frac{\pi}{2^b}}, \forall y \in [1, 2^{b-1}-1] \text{ and}\\
\frac{\partial W^{(b)}_{0}(P',\theta)}{\partial\theta}\Big|_{\theta=\frac{\pi}{2^b}} =& 0
\end{aligned}
$$

By combining this with Lemma 1.ii, (11) becomes 0. Alternatively, we can write (11) as

$$
\begin{aligned}
\frac{\partial\mathcal{L}(\theta)}{\partial\theta} = \sum_{y=1}^{y=2^{b-1}-1}&\left\{\frac{\partial W^{(b)}_{2^{b-1}-y}(P',\theta)}{\partial\theta}\log\left[\frac{W^{(b)}_{2^{b-1}}(P',\theta)}{W^{(b)}_{2^{b-1}-y}(P',\theta)}\right]\right.\\
&\left.+\frac{\partial W^{(b)}_{2^{b-1}-1+y}(P',\theta)}{\partial\theta}\log\left[\frac{W^{(b)}_{2^{b-1}}(P',\theta)}{W^{(b)}_{2^{b-1}-1+y}(P',\theta)}\right]\right\}\\
&+\frac{\partial W^{(b)}_{2^{b-1}-1}(P',\theta)}{\partial\theta}\log\left[\frac{W^{(b)}_{2^{b-1}}(P',\theta)}{W^{(b)}_{2^{b-1}-1}(P',\theta)}\right].
\end{aligned}
\tag{13}
$$

Suppose we have $\theta = 0$. The last term becomes zero due to Lemma 1.iii. We apply Leibniz integral rule to get

$$
\begin{aligned}
\frac{\partial W^{(b)}_{2^{b-1}-y}(P',\theta)}{\partial\theta}\Big|_{\theta=0} =& p_{\Phi|A}\left(-\frac{2\pi y}{2^b}\Big|P'\right) - p_{\Phi|A}\left(-\frac{2\pi(y-1)}{2^b}\Big|P'\right)\\
\frac{\partial W^{(b)}_{2^{b-1}-1+y}(P',\theta)}{\partial\theta}\Big|_{\theta=0} =& p_{\Phi|A}\left(\frac{2\pi(y-1)}{2^b}\Big|P'\right) - p_{\Phi|A}\left(\frac{2\pi y}{2^b}\Big|P'\right)
\end{aligned}
$$

Due to even-symmetry of $p_{\Phi|A}(\phi|\alpha)$, we have

$$
\frac{\partial W^{(b)}_{2^{b-1}-y}(P',\theta)}{\partial\theta}\Big|_{\theta=0} = -\frac{\partial W^{(b)}_{2^{b-1}-1+y}(P',\theta)}{\partial\theta}\Big|_{\theta=0}, \forall y \in [1, 2^{b-1}]
$$

By combining this with Lemma 1.iii, equation (11) becomes 0. Thus, the two stationary points occur at $\theta \in \{0, \frac{\pi}{2^b}\}$. To prove that $\theta = 0$ is not a minimizer, it suffices to show that

$$
\mathcal{L}(0) \geq \mathcal{L}\left(\frac{\pi}{2^b}\right)
$$

$$-\sum_{y=0}^{2^b-1} W_y^{(b)}(P',0)\log W_y^{(b)}(P',0) \geq -\sum_{y=0}^{2^b-1} W_y^{(b)}\left(P',\frac{\pi}{2^b}\right)\log W_y^{(b)}\left(P',\frac{\pi}{2^b}\right)$$

$$2\sum_{y=0}^{2^{b-1}-1} W_y^{(b)}(P',0)\log\frac{1}{W_y^{(b)}(P',0)} \geq \sum_{y=0}^{2^{b-1}-1}\left\{W_{y+1}^{(b)}\left(P',\frac{\pi}{2^b}\right)\log\frac{1}{W_{y+1}^{(b)}\left(P',\frac{\pi}{2^b}\right)} + W_y^{(b)}\left(P',\frac{\pi}{2^b}\right)\log\frac{1}{W_y^{(b)}\left(P',\frac{\pi}{2^b}\right)}\right\},$$

where the LHS follows from Lemma 1.iii and the RHS follows from Lemma 1.ii and the circular structure of the phase quantizer. Since $p_{\Phi|A}(\phi|\alpha)$ is non-decreasing function of $\phi$ for $\phi < 0$, it is easy to verify that

$$W_y^{(b)}(P',0) \leq W_{y+1}^{(b)}\left(P',\frac{\pi}{2^b}\right) \text{ and } W_y^{(b)}(P',0) \geq W_y^{(b)}\left(P',\frac{\pi}{2^b}\right), \qquad \forall y \in [0, 2^{b-1}-1]$$

If we let

$$a_y = W_y^{(b)}(\alpha^*,0),\ a_y - b_y = W_y^{(b)}(\alpha^*,\pi/2^b) \text{ and } a_y + c_y = W_{y+1}^{(b)}(\alpha^*,\pi/2^b)$$

and apply Lemma 7 in Section I, then $\theta = 0$ is actually a maximizer and not a minimizer. Noting that the input distribution should be $\frac{2\pi}{2^b}$-symmetric concludes the proof. □

## I. Breaking Ties in Probabilities Increases Entropy

We prove the following lemma about the entropy of a discrete distribution. Essentially, this lemma tells us that if the distribution has a form $\{p_i\}_{i=1}^{i=N}$ such that $p_i = p_{\frac{N}{2}+i}\ \forall i \in [1, N/2]$, then breaking these ties in the probabilities reduces entropy.

**Lemma 7.** *For all $a_y > 0$ such that $\sum_y a_y = 0.5$, the inequality*

$$-\sum_y (a_y - b_y)\log(a_y - b_y) + (a_y + c_y)\log(a_y + c_y) \leq -2\sum_y a_y \log a_y \tag{14}$$

*holds for all $c_y \geq 0$ and $b_y \geq 0$ that satisfy $\sum_y c_y = \sum_y b_y$.*

*Proof.* Let $f(\boldsymbol{b},\boldsymbol{c})$ be the RHS of (14). The second-order derivatives of $f(\boldsymbol{b},\boldsymbol{c})$ with respect to $b_1$ and $b_2$ are

$$\frac{\partial^2 f(\boldsymbol{b},\boldsymbol{c})}{\partial b_y^2} = -\frac{1}{a_y - b_y} \quad \text{and} \quad \frac{\partial^2 f(\boldsymbol{b},\boldsymbol{c})}{\partial c_y^2} = -\frac{1}{a_y + c_y}, \quad \frac{\partial^2 f(\boldsymbol{b},\boldsymbol{c})}{\partial b_y b_{i\neq y}} = \frac{\partial^2 f(\boldsymbol{b},\boldsymbol{c})}{\partial c_y c_{i\neq y}} = 0,$$

which are all non-positives $b_y$, $c_y$ in the domain of $f(\boldsymbol{b},\boldsymbol{c})$. Thus, $f(\boldsymbol{b},\boldsymbol{c})$ is concave. Next, we construct the Lagrangian as

$$f(\boldsymbol{b},\boldsymbol{c},\lambda) = -\sum_k \left[(a_y - b_y)\log(a_y - b_y) + (a_y + c_y)\log(a_y + c_y)\right] - \lambda\left(\sum_y c_y - b_y\right), \qquad \lambda > 0$$

and the optimal solution $(\boldsymbol{b}^*, \boldsymbol{c}^*)$ should satisfy

$$\frac{\partial f(\boldsymbol{b},\boldsymbol{c},\lambda)}{\partial b_y} = [\log(a_y - b_y) + 1] + \lambda = 0, \qquad \frac{\partial f(\boldsymbol{b},\boldsymbol{c},\lambda)}{\partial c_y} = -[\log(a_y + c_y) + 1] - \lambda = 0.$$

Combining the two stationarity conditions, we get

$$\begin{aligned}[\log(a_y - b_y) + 1] - [\log(a_y + c_y) + 1] =& 0 \\ \log(a_y - b_y) =& \log(a_y + c_y),\end{aligned}$$

which is only satisfied if $c_y = b_y = 0$. Thus, $\boldsymbol{b}^* = \mathbf{0}$ and $\boldsymbol{c}^* = \mathbf{0}$. Plugging $\boldsymbol{b}^*$ and $\boldsymbol{c}^*$ to the LHS of (14) gives the RHS of (14). ☐

## J. Regions where $p_{\Phi|A}(\phi|\alpha)$ is decreasing

In this section, we identify regions for which $p_{\Phi|A}(\phi|\alpha)$ is decreasing.

**Lemma 8.** *The conditional pdf $p_{\Phi|A}(\phi|\alpha)$ is a decreasing function of $\alpha$ for the following cases:*

$$\begin{aligned}&(A) : \phi \in (\pi/2, \pi] \cup [-\pi, -\pi/2) \\ &(B) : \phi \in [-\pi/2, \pi/2] \text{ and } \alpha \geq \frac{1}{2\sin^2\phi}\end{aligned}$$

*Proof.* The first-order derivative of $p_{\Phi|A}(\phi|\alpha)$ with respect to $\alpha$ is

$$\frac{\partial p_{\Phi|A}(\phi|\alpha)}{\partial \alpha} = -\frac{e^{-\alpha}\sin^2\phi}{2\pi} + \frac{e^{-\alpha\sin^2\phi} Q\left(-\sqrt{2\alpha}\cos\phi\right)\cos\phi}{2\sqrt{\alpha}\sqrt{\pi}}(1 - 2\alpha\sin^2\phi). \tag{15}$$

This derivative is analyzed under two scenarios.

**Scenario A ($\phi \in (\pi/2, \pi] \cup [-\pi, -\pi/2)$):**
In this case, $\cos(\phi) < 0$ and we have

$$\frac{\partial p_{\Phi|A}(\phi|\alpha)}{\partial \alpha} = -\underbrace{\frac{e^{-\alpha}\sin^2\phi}{2\pi}}_{>0} - \underbrace{\frac{e^{-\alpha\sin^2\phi} Q\left(-\sqrt{2\alpha}\cos\phi\right)(-\cos\phi)}{2\sqrt{\alpha}\sqrt{\pi}}}_{>0}(1 - 2\alpha\sin^2\phi)$$

which is negative for all $\alpha \leq \frac{1}{2\sin^2\phi}$. For $\alpha > \frac{1}{2\sin^2\phi}$, we have

$$\begin{aligned}\frac{\partial p_{\Phi|A}(\phi|\alpha)}{\partial \alpha} &= -\frac{e^{-\alpha}\sin^2\phi}{2\pi} + \frac{e^{-\alpha\sin^2\phi} Q\left(-\sqrt{2\alpha}\cos\phi\right)(-\cos\phi)}{2\sqrt{\alpha}\sqrt{\pi}}(2\alpha\sin^2\phi - 1) \\ &< -\frac{e^{-\alpha}\sin^2\phi}{2\pi} + \frac{e^{-\alpha\sin^2\phi}\cos\phi}{2\sqrt{\alpha}\sqrt{\pi}} \cdot \frac{e^{-\alpha\cos^2\phi}}{\sqrt{2\pi}(\sqrt{2\alpha}\cos\phi)}(2\alpha\sin^2\phi - 1) \\ &= -\frac{e^{-\alpha}\sin^2\phi}{2\pi} + \frac{e^{-\alpha}}{4\pi\alpha}(2\alpha\sin^2\phi - 1) \\ &= -\frac{e^{-\alpha}}{4\pi\alpha}.\end{aligned}$$

The inequality in the second line comes from the Q-function upper bound $Q(x) < \frac{e^{-\frac{x^2}{2}}}{\sqrt{2\pi}x}$ and the third and fourth lines are obtained through simplification. This shows that (15) is negative in Scenario A.

**Scenario B ($\phi \in [-\pi/2, \pi/2]$):**
In this case, $\cos(\phi) > 0$ and we have In this case, $\cos(\phi) > 0$ and we have

$$\frac{\partial p_{\Phi|A}(\phi|\alpha)}{\partial \alpha} = -\frac{e^{-\alpha}\sin^2\phi}{2\pi} + \underbrace{\frac{e^{-\alpha\sin^2\phi}\left[1 - Q\left(\sqrt{2\alpha}\cos\phi\right)\right]\cos\phi}{2\sqrt{\alpha}\sqrt{\pi}}}_{>0}(1 - 2\alpha\sin^2\phi).$$

The second term is negative if $\alpha \geq \frac{1}{2\sin^2\phi}$. Combining the results from both scenarios completes the proof. □

## K. The function $W^{(b)}_{2^{b-1}}(\alpha, \theta)$ is increasing on $\alpha$ for $b \geq 3$

To prove that $W^{(b)}_{2^{b-1}}(\alpha, \theta)$ is an increasing function of $\alpha$, we need to show that

$$\begin{aligned} \frac{\partial W^{(b)}_{2^{b-1}}(\alpha, \theta)}{\partial \alpha} &= \int_{-\theta}^{\frac{2\pi}{2^b}-\theta} \frac{\partial p_{\Phi|A}(\phi|\alpha)}{\partial \alpha}\, d\phi \\ &= 2\int_0^{\theta} \frac{\partial p_{\Phi|A}(\phi|\alpha)}{\partial \alpha}\, d\phi + \int_{\theta}^{\frac{2\pi}{2^b}-\theta} \frac{\partial p_{\Phi|A}(\phi|\alpha)}{\partial \alpha}\, d\phi, \end{aligned} \tag{16}$$

where $\frac{\partial p_{\Phi|A}(\phi|\alpha)}{\partial \alpha}$ is given in (15), is non-negative. The first integral term in the last equality of (16) follows from the even symmetry property of $\partial_{\Phi|A}(\phi|\alpha)$. We first analyze a simple lower bound of the first term of (16) for arbitrary $\theta$ and show that it is positive for $b \geq 3$. We breakdown the problem into two regions of $\alpha$.

**Region 1** ( $\alpha \in \left[\frac{1}{2\sin^2\theta}, +\infty\right)$ ): We first give a lower bound of $\frac{\partial p_{\Phi|A}(\phi|\alpha)}{\partial \alpha}$ for $\alpha > \frac{1}{2\sin^2\phi}$.

$$\begin{aligned} \frac{\partial p_{\Phi|A}(\phi|\alpha)}{\partial \alpha} >& -\frac{e^{-\alpha\sin^2\phi}\cos\phi(2\alpha\sin^2\phi - 1)}{2\sqrt{\alpha}\sqrt{\pi}} \cdot \left[1 - \frac{e^{-\alpha\cos^2\phi}}{\sqrt{2\pi}\sqrt{2\alpha}\cos\phi}\left(1 - \frac{1}{2\alpha\cos^2\phi}\right)\right] \\ &- \frac{e^{-\alpha}\sin^2\phi}{2\pi} \\ =& -\frac{e^{-\alpha\sin^2\phi}\cos\phi(2\alpha\sin^2\phi - 1)}{2\sqrt{\alpha}\sqrt{\pi}} - \frac{e^{-\alpha}}{4\pi\alpha}\left(1 - \frac{1}{2\alpha\cos^2\phi}\right) - \frac{e^{-\alpha}\tan^2\phi}{4\pi\alpha} \\ =& \frac{e^{-\alpha\sin^2\phi}\cos\phi(1 - 2\alpha\sin^2\phi)}{2\sqrt{\alpha}\sqrt{\pi}} - \frac{e^{-\alpha}\sec^2\phi}{4\pi\alpha}\left(1 - \frac{1}{2\alpha}\right). \end{aligned}$$

The first line is obtained using the Q-function lower bound $Q(x) > \frac{\exp(-x^2/2)}{\sqrt{2\pi}x}\left(1 - \frac{1}{x^2}\right)$. The second and third lines are obtained after some algebraic manipulation. Meanwhile, for $\alpha \leq \frac{1}{2\sin^2\phi}$, the lower bound becomes

$$\begin{aligned} \frac{\partial p_{\Phi|A}(\phi|\alpha)}{\partial \alpha} >& -\frac{e^{-\alpha}\sin^2\phi}{2\pi} + \frac{e^{-\alpha\sin^2\phi}\cos\phi(1 - 2\alpha\sin^2\phi)}{2\sqrt{\alpha}\sqrt{\pi}}\left[1 - \frac{e^{-\alpha\cos^2\phi}}{\sqrt{2\pi}\sqrt{2\alpha}\cos\phi}\right] \\ =& \frac{e^{-\alpha\sin^2\phi}\cos\phi(1 - 2\alpha\sin^2\phi)}{2\sqrt{\alpha}\sqrt{\pi}} - \frac{e^{-\alpha}}{4\pi\alpha}. \end{aligned}$$

The inequality is obtained using the Q-function upper bound $Q(x) < \frac{\exp(-x^2/2)}{\sqrt{2\pi}x}$. Suppose we define $\theta_0 = \sin^{-1}\left(\frac{1}{\sqrt{2\alpha}}\right) \in [0,\theta)$ for some fixed $\alpha$. Then,

$$\begin{aligned}\int_0^\theta \frac{\partial p_{\Phi|A}(\phi|\alpha)}{\partial\alpha}\, d\phi &> \int_{\theta_0}^\theta \left[\frac{e^{-\alpha\sin^2\phi}\cos\phi(1-2\alpha\sin^2\phi)}{2\sqrt{\alpha}\sqrt{\pi}} - \frac{e^{-\alpha}\sec^2\phi}{4\pi\alpha}\left(1-\frac{1}{2\alpha}\right)\right] d\phi \\ &\quad + \int_0^{\theta_0}\left[\frac{e^{-\alpha\sin^2\phi}\cos\phi(1-2\alpha\sin^2\phi)}{2\sqrt{\alpha}\sqrt{\pi}} - \frac{e^{-\alpha}}{4\pi\alpha}\right] d\phi. \\ &= \frac{e^{-\alpha}\left[\tan(\theta_0)-\tan\theta\right]}{4\pi\alpha}\left(1-\frac{1}{2\alpha}\right) - \frac{e^{-\alpha}\theta_0}{4\pi\alpha} + \frac{\sin\theta e^{-\alpha\sin^2\theta}}{2\sqrt{\alpha}\sqrt{\pi}} \\ &= \frac{e^{-\frac{1}{2}\csc^2\theta_0}\sin^2(\theta_0)\cos^2(\theta_0)\left[\tan(\theta_0)-\tan(\theta)\right]}{2\pi} \\ &\quad - \frac{e^{-\frac{1}{2}\csc^2\theta_0}\theta_0\sin^2\theta_0}{2\pi} + \frac{\sqrt{2\pi}\sin(\theta_0)\sin(\theta)\exp\left(-\frac{\sin^2(\theta)}{2\sin^2(\theta_0)}\right)}{2\pi}.\end{aligned}$$

The second line is obtained by evaluating the integrals while the third line follows from expressing the $\alpha$'s in terms of $\theta_0$. We want to show that the above expression is positive. Equivalently, the claim is proven for Region 1 by showing that

$$\sqrt{2\pi}\sin(\theta)\exp\left(\frac{\cos^2(\theta)}{2\sin^2(\theta_0)}\right) \geq \sin\theta_0\left[\theta_0 - \cos^2(\theta_0)\left[\tan(\theta_0)-\tan(\theta)\right]\right] \tag{17}$$

holds for $\theta \in [0, \frac{\pi}{4})$ and $\theta_0 \in [0,\theta]$. At $\theta_0 = \theta$, (17) becomes

$$\sqrt{2\pi}\sin\theta\exp\left(\frac{\cot^2\theta}{2}\right) \geq \theta\sin\theta,$$

which holds for $\theta = [0, \frac{\pi}{4})$. Moreover, for a fixed $\theta$, The LHS of (17) increases as $\theta_0$ moves towards 0. The RHS of (17) can be verified to be an increasing function of $\theta_0$ for $\theta \in [0, \frac{\pi}{4})$ by inspecting its derivative with respect to $\theta_0$. That is,

$$\cos\theta_0[\tan(\theta_0)-\tan(\theta)][2\sin^2(\theta_0)-\cos^2(\theta)] + \theta_0\cos\theta_0 \ > \ 0 \qquad \forall\theta_0 \leq \theta \text{ and } \forall\theta \in [0, \frac{\pi}{4}).$$

As such, the RHS of (17) decreases as $\theta_0$ moves towards 0. The claim holds for region 1.

**Region 2** ( $\alpha \in [0, \frac{1}{2\sin^2\theta})$ ): Similar to Region 1, we give a lower bound of $\frac{\partial p_{\Phi|A}(\phi|\alpha)}{\partial\alpha}$ for $\alpha < \frac{1}{2\sin^2\phi}$. This lower bound is written as

$$\frac{\partial p_{\Phi|A}(\phi|\alpha)}{\partial\alpha} \geq -\frac{e^{-\alpha}\sin^2\phi}{2\pi} + \frac{e^{-\alpha\sin^2\phi}\cos\phi(1-2\alpha\sin^2\phi)}{2\sqrt{\alpha}\sqrt{\pi}}\left[1-\frac{e^{-\alpha\cos^2\phi}}{2}\right]$$

where the inequality is obtained using the Q-function upper bound $Q(x) < \frac{\exp(-x^2/2)}{2}$. Consequently,

$$\int_0^\theta \frac{\partial p_{\Phi|A}(\phi|\alpha)}{\partial\alpha}\, d\phi \geq \int_0^\theta\left[-\frac{e^{-\alpha}\sin^2\phi}{2\pi} + \frac{e^{-\alpha\sin^2\phi}\cos\phi(1-2\alpha\sin^2\phi)}{2\sqrt{\alpha}\sqrt{\pi}}\left[1-\frac{e^{-\alpha\cos^2\phi}}{2}\right]\right] d\phi$$

$$= -\frac{e^{-\alpha}}{4\pi\sqrt{\alpha}}\Bigg[\sqrt{\alpha}\theta - \frac{2\sqrt{\pi}\alpha\sin^3\theta}{3} - \sqrt{\alpha}\sin\theta\cos\theta - 2\sqrt{\pi}\sin\theta e^{\alpha\cos^2\theta} + \sqrt{\pi}\sin\theta\Bigg].$$

We want to show that the above expression is positive. Equivalently, the claim is proven for Region 2 by showing that

$$2\sin\theta e^{\alpha\cos^2\theta} + \frac{2\alpha\sin^3\theta}{3} \geq \sqrt{\frac{\alpha}{\pi}}\left[\theta - \sin\theta\cos\theta\right] + \sin\theta \tag{18}$$

holds for all $\alpha \in [0, \frac{1}{2\sin^2\theta})$. At $\alpha = 0$, we have

$$2\sin\theta \geq \sin\theta$$

which is satisfied for all $\theta$ considered. Both sides increase with $\alpha$ but the LHS increases at a faster rate than the RHS. At the endpoint $\alpha = \frac{1}{2\sin^2\theta}$, we have

$$2\sin\theta e^{\cot^2\theta} \geq \sqrt{\frac{1}{2\pi}}\left[\frac{\theta}{\sin\theta} - \cos\theta\right] + \frac{2\sin\theta}{3}$$

which holds for $\theta \in [0, \frac{\pi}{4})$. Combining the results for both Region 1 and Region 2 shows that the first integral term of (16) is positive. Going back to (16), we have

$$\begin{aligned}\frac{\partial W^{(b)}_{2^{b-1}}(\alpha,\theta)}{\partial\alpha} &= 2\underbrace{\int_0^{\theta}\frac{\partial p_{\Phi|A}(\phi|\alpha)}{\partial\alpha}\,d\phi}_{>0} + \int_{\theta}^{\frac{2\pi}{2^b}-\theta}\frac{\partial p_{\Phi|A}(\phi|\alpha)}{\partial\alpha}\,d\phi \\ &> \int_0^{\theta}\frac{\partial p_{\Phi|A}(\phi|\alpha)}{\partial\alpha}\,d\phi + \int_{\theta}^{\frac{2\pi}{2^b}-\theta}\frac{\partial p_{\Phi|A}(\phi|\alpha)}{\partial\alpha}\,d\phi \\ &= \int_0^{\frac{2\pi}{2^b}-\theta}\frac{\partial p_{\Phi|A}(\phi|\alpha)}{\partial\alpha}\,d\phi,\end{aligned}$$

which is positive when $|\frac{2\pi}{2^b} - \theta| \leq \frac{\pi}{4}$. This is satisfied for $\theta \in [0, \frac{2\pi}{2^b})$ when $b \geq 3$.

## L. Regions where $p_{\Phi|A}(\phi|\alpha)$ has upward curvature

In this section, we identify regions for which $p_{\Phi|A}(\phi|\alpha)$ has upward curvature.

**Lemma 9.** *The conditional pdf $p_{\Phi|A}(\phi|\alpha)$ is a convex function of $\alpha$ for the following cases:*

$$(A): \phi \in (\pi/2, \pi] \cup [-\pi, -\pi/2)$$

$$(B): \phi \in [-\pi/2, \pi/2] \text{ and } \alpha \geq \frac{(1+\sqrt{2})}{2\sin^2\phi}.$$

*Proof.* The second-order derivative of $p_{\Phi|A}(\phi|\alpha)$ with respect to $\alpha$ is

$$\begin{aligned}\frac{\partial^2 p_{\Phi|A}(\phi|\alpha)}{\partial\alpha^2} &= \frac{\partial}{\partial\alpha}\left\{-\frac{e^{-\alpha}\sin^2\phi}{2\pi} + \frac{e^{-\alpha\sin^2\phi}Q\left(-\sqrt{2\alpha}\cos\phi\right)\cos\phi}{2\sqrt{\alpha}\sqrt{\pi}}(1-2\alpha\sin^2\phi)\right\}\\ &=\frac{\cos\phi e^{-\alpha\sin^2\phi}Q\left(-\sqrt{2\alpha}\cos\phi\right)\left[(2\alpha\sin^2\phi-1)^2-2\right]}{4\sqrt{\pi}\alpha^{\frac{3}{2}}}\\ &\quad+\frac{e^{-\alpha}\cos^2\phi}{4\pi\alpha}+\frac{e^{-\alpha}\sin^4\phi}{2\pi}.\end{aligned} \tag{19}$$

We now analyze the two scenarios mentioned in the lemma.

**Scenario A:**
In this case, $\cos(\phi) < 0$ and we have

$$\begin{aligned}\frac{\partial^2 p_{\Phi|A}(\phi|\alpha)}{\partial\alpha^2} &= -\underbrace{\frac{(-\cos\phi)e^{-\alpha\sin^2\phi}Q\left(-\sqrt{2\alpha}\cos\phi\right)}{4\sqrt{\pi}\alpha^{\frac{3}{2}}}}_{>0}\left[(2\alpha\sin^2\phi-1)^2-2\right]\\ &\quad+\frac{e^{-\alpha}\cos^2\phi}{4\pi\alpha}+\frac{e^{-\alpha}\sin^4\phi}{2\pi},\end{aligned}$$

which is negative if $\alpha \leq \frac{1+\sqrt{2}}{2\sin^2\phi}$. For $\alpha > \frac{1+\sqrt{2}}{2\sin^2\phi}$, we have

$$\begin{aligned}\frac{\partial^2 p_{\Phi|A}(\phi|\alpha)}{\partial\alpha^2} &= \underbrace{\frac{(-\cos\phi)e^{-\alpha\sin^2\phi}\left[2-(2\alpha\sin^2\phi-1)^2\right]}{4\sqrt{\pi}\alpha^{\frac{3}{2}}}}_{<0}Q\left(-\sqrt{2\alpha}\cos\phi\right)\\ &\quad+\frac{e^{-\alpha}\cos^2\phi}{4\pi\alpha}+\frac{e^{-\alpha}\sin^4\phi}{2\pi}\\ &>\frac{(-\cos\phi)e^{-\alpha\sin^2\phi}\left[2-(2\alpha\sin^2\phi-1)^2\right]}{4\sqrt{\pi}\alpha^{\frac{3}{2}}}\left[\frac{-e^{-\alpha\cos^2\phi}}{\sqrt{2\pi}\sqrt{2\alpha}\cos\phi}\right]\\ &\quad+\frac{e^{-\alpha}\cos^2\phi}{4\pi\alpha}+\frac{e^{-\alpha}\sin^4\phi}{2\pi}\\ &=\frac{e^{-\alpha}\left[2-(2\alpha\sin^2\phi-1)^2\right]}{8\pi\alpha^2}+\frac{e^{-\alpha}\cos^2\phi}{4\pi\alpha}+\frac{e^{-\alpha}\sin^4\phi}{2\pi},\end{aligned}$$

where the inequality in the second line is obtained using the upper bound $Q(x) < \frac{e^{-\frac{x^2}{2}}}{\sqrt{2\pi}x}$. Further algebraic manipulation leads to the following lower bound:

$$\begin{aligned}\frac{\partial^2 p_{\Phi|A}(\phi|\alpha)}{\partial\alpha^2} &> \frac{e^{-\alpha}}{4\pi\alpha}\left[\frac{1}{2\alpha}+\cos^2\phi\right]-\frac{e^{-\alpha}\sin^4\phi}{2\pi}+\frac{e^{-\alpha}\sin^2\phi}{2\pi\alpha}+\frac{e^{-\alpha}\sin^4\phi}{2\pi}\\ &=\frac{e^{-\alpha}}{4\pi\alpha}\left[\frac{1}{2\alpha}+\cos^2\phi\right]+\frac{e^{-\alpha}\sin^2\phi}{2\pi\alpha}>0.\end{aligned}$$

Combining both regions of $\alpha$ completes the proof that $p_{\Phi|A}(\phi|\alpha)$ is convex $\alpha$ for Scenario A.

**Scenario B:**

In this case, $\cos(\phi) > 0$ and we have

$$\frac{\partial^2 p_{\Phi|A}(\phi|\alpha)}{\partial\alpha^2} = \underbrace{\frac{\cos\phi e^{-\alpha\sin^2\phi} Q\left(-\sqrt{2\alpha}\cos\phi\right)}{4\sqrt{\pi}\alpha^{\frac{3}{2}}}}_{>0} \left[(2\alpha\sin^2\phi - 1)^2 - 2\right] + \frac{e^{-\alpha}\cos^2\phi}{4\alpha\pi} + \frac{e^{-\alpha}\sin^4\phi}{2\pi}.$$

and it is guaranteed that $p_{\Phi|A}(\phi|\alpha)$ is convex on $\alpha$ in this scenario if $\alpha > \frac{1+\sqrt{2}}{2\sin^2\phi}$. □

## M. The function $W^{(b)}_{2^{b-1}}(\alpha,\theta)$ is concave on the parameter $\alpha$ for $b \geq 3$

To prove that $W^{(b)}_{2^{b-1}}(\alpha,\theta)$ is an increasing function of $\alpha$, we need to show that

$$\begin{aligned} \frac{\partial^2 W^{(b)}_{2^{b-1}}(\alpha,\theta)}{\partial\alpha^2} &= \int_{-\theta}^{\frac{2\pi}{2^b}-\theta} \frac{\partial^2 p_{\Phi|A}(\phi|\alpha)}{\partial\alpha^2}\, d\phi \\ &= 2\int_0^{\theta} \frac{\partial^2 p_{\Phi|A}(\phi|\alpha)}{\partial\alpha^2}\, d\phi + \int_{\theta}^{\frac{2\pi}{2^b}-\theta} \frac{\partial^2 p_{\Phi|A}(\phi|\alpha)}{\partial\alpha^2}\, d\phi, \end{aligned} \tag{20}$$

where $\frac{\partial^2 p_{\Phi|A}(\phi|\alpha)}{\partial\alpha^2}$ is given in (19), is non-positive. The first integral term in the last equality of (20) follows from the even-symmetry property of $p_{\phi|A}(\phi|A)$. We first analyze a simple upper bound of the first term of (20) for arbitrary $\theta$ and show that it is positive for $b \geq 3$. We breakdown the problem into two regions of $\alpha$.

**Region 1** ( $\alpha \in \left[\frac{1+\sqrt{2}}{2\sin^2\theta}, +\infty\right)$ ): We first give an upper bound of $\frac{\partial^2 p_{\Phi|A}(\phi|\alpha)}{\partial\alpha^2}$ for $\alpha > \frac{1+\sqrt{2}}{2\sin^2\phi}$.

$$\begin{aligned} \frac{\partial^2 p_{\Phi|A}(\phi|\alpha)}{\partial\alpha^2} <& \frac{\cos\phi e^{-\alpha\sin^2\phi}\left[(2\alpha\sin^2\phi-1)^2-2\right]}{4\sqrt{\pi}\alpha^{\frac{3}{2}}}\left[1 - \frac{e^{-\alpha\cos^2\phi}}{\sqrt{2\pi}\sqrt{2\alpha}\cos\phi}\left(1-\frac{1}{2\alpha\cos^2\phi}\right)\right] \\ &+ \frac{e^{-\alpha}\cos^2\phi}{4\pi\alpha} + \frac{e^{-\alpha}\sin^4\phi}{2\pi} \\ =& \frac{\cos\phi e^{-\alpha\sin^2\phi}\left[(2\alpha\sin^2\phi-1)^2-2\right]}{4\sqrt{\pi}\alpha^{\frac{3}{2}}} + \frac{e^{-\alpha}[1+\sin^2\phi]}{4\pi\alpha} + \frac{e^{-\alpha}}{8\pi\alpha^2} \\ &+ \frac{e^{-\alpha}\left[(2\alpha\sin^2\phi-1)^2-2\right]}{16\pi\alpha^3\cos^2\phi} \end{aligned}$$

The first line follows from using the Q-function lower bound $Q(x) > \frac{\exp(-x^2/2)}{\sqrt{2\pi}x}\left(1-\frac{1}{x^2}\right)$ the second line is obtained after some algebraic manipulation. For $\alpha < \frac{1+\sqrt{2}}{2\sin^2\phi}$, an upper bound can be expressed as

$$\begin{aligned} \frac{\partial^2 p_{\Phi|A}(\phi|\alpha)}{\partial\alpha^2} <& -\frac{\cos\phi e^{-\alpha\sin^2\phi}\left[2-(2\alpha\sin^2\phi-1)^2\right]}{4\sqrt{\pi}\alpha^{\frac{3}{2}}}\left[1 - \frac{e^{-\alpha\cos^2\phi}}{\sqrt{2\pi}\sqrt{2\alpha}\cos\phi}\right] \\ &+ \frac{e^{-\alpha}\cos^2\phi}{4\alpha\pi} + \frac{e^{-\alpha}\sin^4\phi}{2\pi} \end{aligned}$$

$$=\frac{\cos\phi e^{-\alpha\sin^2\phi}\left[(2\alpha\sin^2\phi-1)^2-2\right]}{4\sqrt{\pi}\alpha^{\frac{3}{2}}}+\frac{e^{-\alpha}[1+\sin^2\phi]}{4\alpha\pi}+\frac{e^{-\alpha}}{8\pi\alpha^2}$$

where the inequality is obtained using the Q-function upper bound $Q(x) < \frac{\exp(-x^2/2)}{\sqrt{2\pi}x}$. Suppose we define $\theta_0 = \sin^{-1}\left(\sqrt{\frac{1+\sqrt{2}}{2\alpha}}\right) > 0$. Then,

$$\begin{aligned}\int_0^\theta \frac{\partial^2 p_{\Phi|A}(\phi|\alpha)}{\partial\alpha^2}d\phi <& \int_0^\theta \left[\frac{\cos\phi e^{-\alpha\sin^2\phi}\left[(2\alpha\sin^2\phi-1)^2-2\right]}{4\sqrt{\pi}\alpha^{\frac{3}{2}}}+\frac{e^{-\alpha}[1+\sin^2\phi]}{4\alpha\pi}+\frac{e^{-\alpha}}{8\pi\alpha^2}\right]d\phi\\
&+\int_{\theta_0}^\theta \frac{e^{-\alpha}\left[(2\alpha\sin^2\phi-1)^2-2\right]}{16\pi\alpha^3\cos^2\phi}\,d\phi\\
=&\frac{e^{-\alpha}}{8\pi\alpha^2}\left[(3\alpha+1)\theta-4\sqrt{\pi}\alpha^{\frac{3}{2}}\sin^3\theta e^{\alpha\cos^2\theta}-2\sqrt{\pi}\sqrt{\alpha}\sin\theta e^{\alpha\cos^2\theta}-\frac{\alpha\sin(2\theta)}{2}\right]\\
&+\frac{e^{-\alpha}}{16\pi\alpha^3}\left[(4\alpha^2-4\alpha-1)\tan\theta+\alpha^2\sin(2\theta)+2(2-3\alpha)\alpha\theta\right]\\
&-\frac{e^{-\alpha}}{16\pi\alpha^3}\left[(4\alpha^2-4\alpha-1)\tan\theta_0+\alpha^2\sin(2\theta_0)+2(2-3\alpha)\alpha\theta_0\right].\end{aligned}$$

We want to show that the above expression is negative for $\theta_0 \in [0,\theta]$ and $\theta \in [0,\frac{\pi}{4}]$. Equivalently, by some algebraic manipulation and by expressing the $\alpha$'s in terms of $\theta_0$, the claim is proven for Region 1 by showing that

$$\begin{aligned}3\theta-4\sqrt{\pi}\left(\frac{1+\sqrt{2}}{2}\right)^{\frac{3}{2}}\left(\frac{\sin\theta}{\sin\theta_0}\right)^3 e^{\frac{1+\sqrt{2}}{2}\cot^2\theta}-2\sqrt{\pi}\left(\frac{1+\sqrt{2}}{2}\right)^{\frac{1}{2}}\left(\frac{\sin\theta}{\sin\theta_0}\right)e^{\frac{1+\sqrt{2}}{2}\cot^2\theta}\\
<\left[\frac{1+\sqrt{2}}{\sin^2\theta_0}-\frac{\sin^2\theta_0}{1+\sqrt{2}}-2\right][\tan\theta_0-\tan\theta]+\frac{1+\sqrt{2}}{2}\cot\theta_0+\left[2-\frac{3(1+\sqrt{2})}{2\sin^2\theta_0}\right]\theta_0\end{aligned}$$

A (stricter) inequality can be achieved by using the following lower bound for the first term of the RHS:

$$\left[\frac{1+\sqrt{2}}{\sin^2\theta_0}-\frac{\sin^2\theta_0}{1+\sqrt{2}}-2\right][\tan\theta_0-\tan\theta]\geq\frac{1+\sqrt{2}}{\sin^2\theta_0}[\tan\theta_0-\tan\theta],$$

dropping the third term in the LHS (which is negative), and the second term of the RHS (which is positive). Multiplying boths sides by $\sin^3(\theta_0)$ and rearranging the terms give us

$$\begin{aligned}&3\theta\sin^3\theta_0-\left[2\sin^2\theta_0-\frac{3(1+\sqrt{2})}{2}\right]\theta_0\sin\theta_0\\
&<\sin\theta_0(1+\sqrt{2})[\tan\theta_0-\tan\theta]+4\sqrt{\pi}\left(\frac{1+\sqrt{2}}{2}\right)^{\frac{3}{2}}\sin^3\theta e^{\frac{1+\sqrt{2}}{2}\cot^2\theta}\end{aligned}\tag{21}$$

For $\theta_0 = \theta$, the expression becomes

$$\theta \sin^3\theta + \frac{3(1+\sqrt{2})\theta\sin\theta}{2} < 4\sqrt{\pi}\left(\frac{1+\sqrt{2}}{2}\right)^{\frac{3}{2}} \sin^3\theta e^{\frac{1+\sqrt{2}}{2}\cot^2\theta}$$

which holds for $\theta \in [0, \frac{\pi}{4}]$. Moreover, for a fixed value of $\theta \in [0, \frac{\pi}{4}]$, it can be verified that the LHS of (21) decreases and the RHS of (21) increases as $\theta_0$ moves towards 0. As such, the claim holds for region 1.

**Region 2** ( $\alpha \in [0, \frac{1+\sqrt{2}}{2\sin^2\theta)}$ ): In this region, we first give an upper bound of $\frac{\partial^2 p_{\Phi|A}(\phi|\alpha)}{\partial\alpha^2}$ for $\alpha < \frac{1+\sqrt{2}}{2\sin^2\phi}$. This upper bound can be expressed as

$$\begin{aligned}\frac{\partial^2 p_{\Phi|A}(\phi|\alpha)}{\partial\alpha^2} &\le -\frac{\cos\phi e^{-\alpha\sin^2\phi}\left[2-(2\alpha\sin^2\phi-1)^2\right]}{4\sqrt{\pi}\alpha^{\frac{3}{2}}}\left[1-\frac{e^{-\alpha\cos^2\phi}}{2}\right] \\ &\quad + \frac{e^{-\alpha}\cos^2\phi}{4\alpha\pi} + \frac{e^{-\alpha}\sin^4\phi}{2\pi} \\ &= -\frac{\cos\phi e^{-\alpha\sin^2\phi}\left[2-(2\alpha\sin^2\phi-1)^2\right]}{4\sqrt{\pi}\alpha^{\frac{3}{2}}} + \frac{e^{-\alpha}\cos^2\phi}{4\alpha\pi} \\ &\quad + \frac{e^{-\alpha}\sin^4\phi}{2\pi} + \frac{\cos\phi e^{-\alpha}[2-(2\alpha\sin^2\phi-1)^2]}{8\sqrt{\pi}\alpha^{\frac{3}{2}}}\end{aligned}$$

where the second inequality is obtained using the Q-function upper bound $Q(x) < \frac{\exp(-x^2/2)}{2}$. Consequently, we have

$$\begin{aligned}\int_0^\theta \frac{\partial^2 p_{\Phi|A}(\phi|\alpha)}{\partial\alpha^2}d\phi \le& \frac{e^{-\alpha}}{8\sqrt{\pi}\alpha^{\frac{3}{2}}}\left[\sin\theta - 2\sin\theta e^{\alpha\cos^2\theta} - 4\alpha\sin^3\theta e^{\alpha\cos^2\theta} + \frac{4\alpha\sin^3\theta}{3} - \frac{4\alpha^2\sin^5\theta}{5}\right] \\ &+ \frac{e^{-\alpha}\left[\theta+\sin\theta\cos\theta\right]}{8\pi\alpha} + \frac{e^{-\alpha}(12\theta - 8\sin(2\theta)+\sin(4\theta))}{64\pi}.\end{aligned}$$

We want to show that the above expression is positive. Equivalently, after some algebraic manipulation, the claim is proven for Region 2 by showing that

$$\begin{aligned}\frac{\alpha^{\frac{3}{2}}}{\sqrt{\pi}}\left[\frac{3\theta}{2} - \sin(2\theta) + \frac{\cos(2\theta)\sin(2\theta)}{4}\right] + 4\alpha\sin^3\theta\left[\frac{1}{3} - e^{\alpha\cos^2\theta}\right] \\ + \sin\theta[1-2e^{\alpha\cos^2\theta}] + \sqrt{\frac{\alpha}{\pi}}\left[\theta+\sin\theta\cos\theta\right] < \frac{4\alpha^2\sin^5\theta}{5}\end{aligned} \tag{22}$$

holds for all $\theta \in [0, \frac{\pi}{4}]$ and $\alpha$ in Region 2. At $\alpha = 0$, we have

$$-\sin\theta \le 0$$

which is satisfied for all $\theta \in [0, \frac{\pi}{4})$. Moreover, for any fixed $\theta \in [0, \frac{\pi}{4})$, the RHS of (22) increases as $\alpha$ increases. Only the last term in the LHS of (22) is non-negative and this term grows at a slower rate than the other terms so the LHS of (22) decreases as $\alpha$ increases. As such, the claim holds for Region 2. Combining the results for both Region 2 and Region 1 shows that

the first term of (20) is negative. Going back to (20), we have

$$\begin{aligned}\frac{\partial^2 W^{(b)}_{2^{b-1}}(\alpha,\theta)}{\partial\alpha^2} &= 2\underbrace{\int_0^{\theta} \frac{\partial^2 p_{\Phi|A}(\phi|\alpha)}{\partial\alpha^2}\,d\phi}_{<0} + \int_{\theta}^{\frac{2\pi}{2^b}-\theta} \frac{\partial^2 p_{\Phi|A}(\phi|\alpha)}{\partial\alpha^2}\,d\phi \\ &< \underbrace{\int_0^{\theta} \frac{\partial^2 p_{\Phi|A}(\phi|\alpha)}{\partial\alpha^2}\,d\phi}_{<0} + \int_{\theta}^{\frac{2\pi}{2^b}-\theta} \frac{\partial^2 p_{\Phi|A}(\phi|\alpha)}{\partial\alpha^2}\,d\phi \\ &= \int_0^{\frac{2\pi}{2^b}-\theta} \frac{\partial^2 p_{\Phi|A}(\phi|\alpha)}{\partial\alpha^2}\,d\phi,\end{aligned}$$

which is negative when $|\frac{2\pi}{2^b}-\theta| \leq \frac{\pi}{4}$. This is satisfied for $\theta \in [0, \frac{2\pi}{2^b})$ when $b \geq 3$.

## References


[1] J. Singh, O. Dabeer, and U. Madhow, "On the limits of communication with low-precision analog-to-digital conversion at the receiver." WCSL Technical Report, USCB [Online], Available: `https://wcsl.ece.ucsb.edu/sites/default/files/publications/adc_limits_tech_report.pdf`.

[2] S. Krone and G. Fettweis, "Fading channels with 1-bit output quantization: Optimal modulation, ergodic capacity and outage probability," in *2010 IEEE Information Theory Workshop*, pp. 1–5, 2010.

[3] L. Alaoglu, "Weak topologies of normed linear spaces," *Annals of Mathematics*, vol. 41, no. 1, pp. 252–267, 1940.

[4] T. M. Cover and J. A. Thomas, *Elements of Information Theory (Wiley Series in Telecommunications and Signal Processing)*. USA: Wiley-Interscience, 2006.

[5] L. E. Dubins, "On extreme points of convex sets," *Journal of Mathematical Analysis and Applications*, vol. 5, no. 2, pp. 237 – 244, 1962.

[6] H. Witsenhausen, "Some aspects of convexity useful in information theory," *IEEE Transactions on Information Theory*, vol. 26, no. 3, pp. 265–271, 1980.
